# Supplementary material for: Non-Contact Monitoring of Dehydration using RF Data Collected off the Chest and the Hand
Source: arXiv:2306.10130 source file (2023-06-16)
Supplement: Supplementary file 1 [file appendix.tex]

\section{}
